# Supplementary material for: A workload-adaptive mechanism for linear queries under local differential privacy
Source: arXiv:2002.01582 source file (2020-05-18)
Supplement: Supplementary file 1 [file appendix2.tex]

\begin{table*}[t]
\centering
\begin{tabular}{| c | c | c | c|} 
 \hline
 Mechanism &Input& Output & Strategy Matrix \\ 
 \hline 
 \hline
 \textbf{Randomized Response}~\cite{warner1965randomized}& $ u \in [n] $ &  $o \in [n] $ & $ \Q_{ou} \propto
\begin{cases} 
\exp{(\epsilon)} & o = u \\
1 & o \neq u 
\end{cases} $ \\
 \hline
 \textbf{RAPPOR}~\cite{erlingsson2014rappor}& \makecell {$u \in [n] $}& $ o \in \{0,1\}^n $ & $
\Q_{ou} = \Big(\frac{1}{1 + \exp{(\epsilon/2)}}\Big)^{|| o - e_u ||_1}   \Big(\frac{\exp{(\epsilon/2)}}{1 + \exp{(\epsilon/2)}}\Big)^{n - || o - e_u ||_1}
$\\
\hline
\textbf{Hadamard}~\cite{acharya2018} & $u \in [n]$ & \makecell {$o \in [K] $ \\$K=[2^{\lceil\log_2(n+1)\rceil}]$}&  $ \Q_{ou} \propto
\begin{cases} 
\exp{(\epsilon)} & o \in C_u  \\
1 &  o \in [K]/C_u
\end{cases} $ \\
\hline
\textbf{Subset Selection}~\cite{ye2018optimal} & $u \in [n]$ & \makecell {$ o\in \{0,1\}^n$ \\ $\|o\|_{\ell_0}=d $} &$ \Q_{ou} \propto
\begin{cases} 
\exp{(\epsilon)} & o_u = 1 \\
1 &  o_u = 0
\end{cases} $ \\
\hline
\end{tabular}
\text{$e_u$ is the one-hot encoding of $u$.  $C_{u} :$ is the index of the $1$-s in the $(u+1)$th column of the $K\times K$ Hadamard matrix.  }
\caption{Existing LDP mechanisms encoded as a strategy matrix in our framework.}
\label{table:stdmech}
\end{table*}

\begin{table*}[t]
\centering
\begin{tabular}{| c | c | c | c|} 
 \hline
 Mechanism &Input& Output & Estimation \\ 
\hline
Bassiley & $w\in \mathbb{R}^n$ &\makecell{ $\hat{w}=w+\eta \text{ where } \eta \sim \mathcal{N}(0,\sigma^2I_{n\times n})$ \\ $\sigma^2= 2r^2 \log(\frac{2/\delta}{\epsilon^2})  \quad r=\max_{i}\| w_i\|_2$\\ Perform Rejection Sampling for $(\epsilon,0)$ privacy \\  } & \makecell {$ \Tilde{w}=\frac{1}{N}\sum_{i=1}^N \hat{w}_i \quad \text{if   } n> \frac{n^2 \log(2/\delta)}{8 \epsilon^2 \log m}$ \\  else  $ \arg\min_{w\in W\mathbb{B}}\|w- \Tilde{w}\|$  where $\mathbb{B}$ unit $l_1$ ball}  \\
\hline 

Bun & $w\in \mathcal{X} \subset [0,1]^m $ & \makecell{Return $\hat{w}$ using Definition 5.5 cite ;\\ Follow Privacy via max Divergence}  & \makecell {$\bar{W}= \frac{1}{N}\sum_{i=1}^N \hat{w} $ \\  $\arg\min_{w \in \mathcal{X}}\|w- \bar{W}\|$ }\\

\hline 
\end{tabular}
\caption{General Workload Mechanism}
\label{table:Genwork}
\end{table*}

\begin{table*}[h!]
\centering
\begin{tabular}{| c | c | c | c|} 
 \hline
 Mechanism &Input& Output & Privacy \\ 
\hline
Marginal Release & $u \in \{0,1\}^k$ & \makecell {$RR(-1)^{\la u,o \ra} \quad  $ Pick uniformly $o\in \{0,1\}^k$ \\RR: Randomized Response with $\epsilon$ privacy }&  \\
\hline 

Range Query & & & \\

\hline 
\end{tabular}
\caption{Specific Workload Mechanism}
\label{table:Spwork}
\end{table*}

\vspace{1in}

\begin{figure*}[h!]
\begin{tikzpicture}
%\draw (-22,0) rectangle (-15,1) ;
\node[draw,align=left] at (-20,.5) { Problem ~\ref{prob:optimization} \\$ \mathcal{M}^* = \argmin_{\mathcal{M}} \big\{ \max_{D} \mathbb{E}[ \norm{\W \x - \mathcal{M}(\x)}_2^2] \big\}$} ;
\draw[->] (-16.5,.5) --(-14.2,.5);
%\draw (-13,0) rectangle (-5,1) ;
\node at (-15.2,.7) { Worst Case };
\node[draw,align=left] at (-11,.5) { ~\cref{thm:worst-variance}\\ $N \max_{u \in \U} \sum_{i=1}^p \v_i^T \text{Diag}(\q_u) \v_i - (\v_i^T \q_u)^2$};
\draw[->] (-9,0) --(-9,-2.2);
\node at (-9.8,-1.2 ) {relaxation} ;
\node[draw,align=left] at (-9,-2.5) {Claim 3 \\ $L(\V,\Q)=tr[\V \D \V^T] - \norm{\W}_F^2$};
\draw[->] (-11.5,-2.5) -- (-12.7,-3.5);
\draw[->] (-11.5,-2.5) -- (-12.1,-1.5);
\node[draw,align=left] at (-15,-1.5) {Claim 5 \\$L(\Q) = tr[(\Q^T \D^{-1} \Q)^{-1} (\W^T \W)] $};
\node[draw,align=left] at (-15,-3.5) {Claim 4 \\ $ \V = \W (\Q^T \D^{-1} \Q)^{-1} \Q^T \D^{-1} $};
\draw[->] (-15,-2)-- (-15,-3);
\node at (-15.2,-2.5) {Q};
\node[draw] at (-22,-1.5) {$\begin{aligned}
& \underset{\Q, \z}{\text{minimize}}
& & tr[(\Q^T \D^{-1} \Q)^{-1} (\W^T \W) ] \\
& \text{subject to}
& & \Q^T \mathbf{1} = \mathbf{1} \\
& & & \mathbf{0} \leq \z \leq \q_u \leq \exp{(\epsilon)} \z \quad \forall u\\
\end{aligned}$};
\node[draw] at (-22,-3.5) {$\begin{aligned}
& Problem ~\ref{prob:strategyopt} \\
& \underset{\v_i}{\text{minimize}}
& & \v_i^T \D \v_i \\
& \text{subject to}
& & \Q^T \v_i = \w_i 
\end{aligned}$};
\draw[<-> ] (-18.8,-1.5) -- (-17.7,-1.5);
\draw[<-> ] (-20,-3.5) -- (-17.5,-3.5);
\end{tikzpicture}
\caption{\gm{If we keep this drawing, it could be rearranged to be more readable}}
\end{figure*}
